# Supplementary material for: Prior Flow Variational Autoencoder: A density estimation model for Non-Intrusive Load Monitoring
Source: arXiv:2011.14870 source file (2021-06-27)
Supplement: Supplementary file 1 [file abstract.tex]

\begin{abstract}
    
    This document provides supplementary material for the paper entitled 
        -- 
        Prior Flow Variational Autoencoder: 
        A density estimation model for Non-Intrusive Load Monitoring.
    In the following, 
        we provide more detailed information about the results reported in the paper, 
        including per machinery comparison tables for the ablation studies 
        and comparisons of the models' optimization curves for each ablation.
    Additionally,  
        we present visual comparison plots between 
        the ground truth data 
        and the model predictions.
\end{abstract}
