# Supplementary material for: Prior Flow Variational Autoencoder: A density estimation model for Non-Intrusive Load Monitoring
Source: arXiv:2011.14870 source file (2021-06-27)
Supplement: Supplementary file 2 [file results_table.tex]

% \newcolumntype{R}{>{\raggedleft\arraybackslash}X}%
% \newcolumntype{L}[1]{>{\raggedright\arraybackslash}X}%
\begin{table}[ht]
    \caption{
        Performance comparison between the {\ModelName} and the Wavenet (WN) models.
    }
    \label{tab:results}
    \begin{center}
    \begin{small}
    \begin{sc}
    \begin{tabularx}{0.8\columnwidth}{X ll}
        &
            \multicolumn{2}{c}{NDE} \\
        &  
             \multicolumn{1}{c}{WN} 
            %  WN 
        & 
            \multicolumn{1}{c}{{\ModelName}} \\   
            % {\ModelName} \\   
        \bottomrule
        \midrule
        
        PI    & 
            0.045 $\pm$ 0.002  &  {\ndePI} \\
            
        PII    & 
            0.056 $\pm$ 0.002 & {\ndePII} \\
                
        DPCI    & 
            0.08 $\pm$ 0.01  & {\ndeDPCI} \\
        
        DPCII    & 
            0.202 $\pm$ 0.006  & {\ndeDPCII} \\
        
        EFI    & 
            \textbf{0.046 $\pm$ 0.0004}  & {\ndeEFI} \\
            
        EFII    & 
            \textbf{0.041 $\pm$ 0.003}  & {\ndeEFII} \\
            
        MI    & 
            0.08 $\pm$ 0.02  & {\ndeMI} \\
        
        MII    & 
            0.06 $\pm$ 0.01  & {\ndeMII} \\
        \\    
        % \midrule 
        % \toprule
        &
            \multicolumn{2}{c}{SAE} \\
        &  
             \multicolumn{1}{c}{WN}
        & 
            \multicolumn{1}{c}{{\ModelName}} \\
        \bottomrule   
        \midrule
        
        PI    & 
            0.047 $\pm$ 0.009 & {\saePI} \\

        PII    & 
            0.022 $\pm$ 0.009 & {\saePII} \\
                
        DPCI    & 
            0.13 $\pm$ 0.04  & {\saeDPCI} \\
        
        DPCII    & 
            0.19 $\pm$ 0.02  & {\saeDPCII} \\
        
        EFI    & 
            \textbf{0.007 $\pm$ 0.006}  & {\saeEFI} \\
            
        EFII    & 
            \textbf{0.016 $\pm$ 0.009}  & {\saeEFII} \\ 
            
        MI    & 
            0.09 $\pm$ 0.04 & {\saeMI} \\
            
        MII    & 
            \textbf{0.03 $\pm$ 0.02} & {\saeMII} %\\
            
    \end{tabularx}
    \end{sc}
    \end{small}
    \end{center}
    \vskip -0.15in
\end{table}
